# Supplementary material for: On the role of the Barbero-Immirzi parameter in discrete quantum gravity
Source: arXiv:1209.4892 source file (2012-09-21)
Supplement: Supplementary file 1 [file continuum.tex]

 %!TEX root = ../../phase3e.tex

\section{Removing the dependence on $N_i{}^A$ and $P^i{}_A$}
\label{red}

The Plebanski action for gravity is generally formulated on a smooth manifold $\cM$ and may be described by the following action:
\be\label{pleb01}
\cS_{Pleb,\cM}[X, w, \phi] = \frac{1}{2}\int_\cM d^4x \left[ \epsilon^{\lambda\mu\nu\rho}\; <\cP_{\gamma} X_{\lambda\mu}, F[w]_{\nu\rho}> + \frac{1}{2}\,\phi^{\lambda\mu\nu\rho} \prec X_{\lambda\mu}, X_{\nu\rho}\succ\right],
\ee
where $X$ is the bi-vector field, $w$ is a connection, $F$ is its curvature, $\cP_\gamma : \so(4) \rightarrow \so(4) = \delta + \frac{1}{\gamma}\epsilon$ and $\gamma$ is the Barbero-Immirzi parameter.  $\epsilon^{\lambda\mu\nu\rho}$ is a spacetime density, while $<\,,>$ and $\prec\,,\succ$ are two bilinear forms on $\so(4)$, about which we give more details in Appendix \ref{conv}. We have introduced a co-ordinate chart labelled by $x^\mu = (t, x^i)$, where $\mu \in \{0,\,1,\,2,\,3\}$ and $i\in\{1,\,2,\,3\}$.  The first term in the action describes a topological theory known as $BF$ theory (with Holst modification \cite{holst}). The Lagrange multiplier $\phi^{\lambda\mu\nu\rho}$ is a symmetric traceless matrix in the the sense that: $\phi^{\lambda\mu\nu\rho} = \phi^{[\lambda\mu][\nu\rho]} = \phi^{[\nu\rho][\lambda\mu]}$ and $\epsilon_{\lambda\mu\nu\rho}\,\phi^{\lambda\mu\nu\rho} = 0$ and variation with respect to it imposes the simplicity constraints:
\be\label{pleb02}
\prec X_{\lambda\mu}, X_{\nu\rho}\succ\, = \frac V{4!}\; \epsilon_{\lambda\mu\nu\rho} ,\quad\quad\mathrm{where}\quad\quad V = \epsilon^{\lambda\mu\nu\rho} \prec X_{\lambda\mu}, X_{\nu\rho}\succ.
\ee
The quantity denoted $V$ is ultimately a multiple of the 4-volume functional on geometric configurations.  The non-degenerate class of solutions to these constraints  falls into two sectors.  More precisely, if $V \neq 0$, then:
\be\label{pleb03}
X_{\lambda\mu}^A = \left\{
\ba{l}
\pm\;(e_\lambda\, e_\mu)^A,\\[0.1cm]
\pm\; \epsilon^A{}_B\; (e_\lambda\, e_\nu)^B,
\ea\right.
\ee
where $e_\lambda{}^a$ is a co-frame field and $(e\, f)^A = e^{[a}\,f^{b]}$. The index $A=a\bar{a}$ is anti-symmetric in $a$ and $\bar{a}$, with $a,\bar{a}\in\{0,\,1,\, 2,\,3\}$.    These solution sets are referred to as topological and gravitational, respectively.  For $\gamma= \infty$, it is well known that substituting the topological solutions back into the action \eqref{pleb01} produces an action that may be written as a total divergence, while if one substitutes for the gravitational solution set, one arrives at the Palatini action for general relativity.  For finite Immirzi parameter, one cannot maintain such strict distinctions since both sets of solutions give a mix of topological and gravitational actions, but one keeps the nomenclature in any case.

Our interest lies in performing a canonical analysis of this theory.  On a smooth manifold, this has been done in detail in \cite{henneaux}.  Although our analysis shall overlap significantly in the beginning, we shall depart at some point to investigate a discrete version of the theory.   We give some pertinent highlights of the continuum theory here but we refer the reader to \cite{henneaux} for all the details. 

Firstly, we shall assume that the manifold is foliable:  $\cM = \R \times \Sigma$ and that we have already been astute enough to choose a suitable chart. The dynamical variables are the canonical pairs: $(w_i{}^A, \cP_\gamma\Pi^i{}_A)$ and $(\cP_\gamma N_i{}^A, P^i{}_A)$ where we define $\Pi^i{}_A := \epsilon^{ijk}\;\delta_{AB}\;X_{jk}{}^{B}$, $N_i{}^A = X_{0i}{}^A$  and $P^i{}_A$ is a canonical momentum introduced for the variables $N_i{}^A$ to facilitate the canonical reduction.\footnote{A priori, $N_i{}^A$ does not occur with a time derivative in the original action, but it does occur quadratically which obstructs its treatment as a Lagrange multiplier.}  The symplectic structure on the unreduced phase space is:
\be
\label{pleb04}
\{w_i{}^A, \cP_\gamma\Pi^j{}_B\}  = \delta_i{}^j\; \delta^A{}_B, \quad\quad \{\cP_\gamma N_i^A, P^j{}_B\} = \delta_i{}^j\; \delta^A{}_B,
\ee
while the Hamiltonian density is:
\be
\label{pleb05}
\ba{rcl}
\cH &:=&\dsty  - <\cP_\gamma N_i, F^i> - <w_0,  D_i (\cP_{\gamma}\Pi^i)> - <\mu_i, P^i>\\ [0.3cm]
&& \dsty \quad\quad -\, \bar \Phi{}^{ij} \prec N_i{}, N_j\succ -\, \Phi{}^i{}_j \prec N_i, \Pi^j\succ -\,  \hat \Phi{}_{ij} \prec \Pi^i,\Pi^j\succ , 
\ea
\ee
where $[\,\cdot,\cdot\,]$ is the bracket on the Lie algebra. We tacitly assume spatial dependence of both the Poisson brackets and Hamiltonian density. Notice that we have introduced the term $<\mu_i, P^i>$ to ensure the vanishing of the momentum conjugate to $\cP_\g N_i{}^A$.  Moreover, we have made the following definitions for Lagrange multipliers:  $\bar \Phi^{ij} := \phi^{0i0j}$, $\Phi^i{}_j := \frac12\,\epsilon_{jmn}\,\phi^{0imn}$ and $\hat \Phi_{ij} := \frac{1}{16}\,\epsilon_{ikl}\;\epsilon_{jmn}\;\phi^{klmn}$, where the traceless condition now takes the form $\Phi^i{}_i = 0$.

Let us summarise the results of a constraint analysis.
\begin{description}
\item[Gauss constraint:] There are 6 primary first class constraints:
\be
\label{pleb06}
\cG^A =  D_i (\cP_{\gamma}\Pi^i)^A + [\cP_\gamma N_i,\,P^i]^A.
\ee
Note that we have added a term which is zero on the primary constraint surface (to ensure that all the dynamical variables are rotated, that is, so that it is truly first class).  The Gauss constraint is preserved under Hamiltonian evolution.  

\item[$P$ constraint:] The primary constraint: $P^i{}_A \approx 0$ contains 18 equations, 4 of which are first class and 14 of which are second class:
\be
\label{pleb07}
\ba{rcl}
\kappa_0 & = & <\cP_\g N_i, P^i > ,\\[0.2cm]
\kappa_i & = & \epsilon_{ijk} <\cP_\g\Pi^j, P^k> , \\[0.2cm]
\Phi(N_i,P^j) & = &<\cP_\g N_i, P^j> - \frac13\; \delta_i{}^j <\cP_\g N_k, P^k> , \\[0.2cm]
\Phi(\Pi^i, P^j) &=& <\cP_\g\Pi^{(i}, P^{j)}> .
\ea
\ee
We denote by $\kappa_0$ and $\kappa_i$ the first class components.  Hamiltonian evolution generates 18 more equations $\dot P_i{}^A \approx 0$, 4 of which are once again first class constraints and 14 of which determine the 14 Lagrange multipliers $\bar\Phi^{ij}$ and $\Phi^i{}_j$.  The secondary first class constraints are:
\be
\label{pleb08}
\ba{rcl}
\lambda_0 & = & <\cP_\g N_i, F^i>  ,\\[0.2cm]
\lambda_i & = & \epsilon_{ijk} <\cP_\g\Pi^j,F^k> .
\ea
\ee
As a note, they are not first class in their current state but can be rendered in such a form by the subtracting a linear combination of second class constraints.

\item[Simplicity constraints:] The 20 constraints we saw in the Lagrangian formulation arise as primary simplicity constraints in the canonical analysis:
\be
\label{pleb09}
\ba{lcl}
\Phi(N_i,N_j) &=& \prec N_i,  N_j\succ,\\[0.2cm]
\Phi(N_i,\Pi^j) &=& \prec N_i, \Pi^j\succ - \frac{1}{3}\; \delta_i{}^j\; V, \\[0.2cm]
\Phi(\Pi^i,\Pi^j) &=& \prec \Pi^i,\Pi^j\succ.
\ea
\ee
Note that since these constraints depend on only half of each canonical pair, they commute amongst themselves with respect to the Poisson bracket but we shall see shortly that they are all second class. Evolution of $\Phi(N, N)$ and $\Phi(N,\Pi)$ generate 14 equations which determine the Lagrange multipliers $\mu_i$ corresponding the 14 second class components of $P^i$.   However, upon demanding the preservation in time of $\Phi(\Pi,\Pi)$, one generates 6 secondary simplicity constraints:
\be
\label{pleb10}
\Psi^{ij} = \dot \Phi(\Pi^i,\Pi^j) = \epsilon^{mn(i} \prec\cP_\g N_m,  D_n \Pi^{j)}\succ.
\ee
These do not commute with the primary simplicity constraints and thus are also second class.  Iterating the evolution procedure once more, one arrives at 6 equations $\dot \Psi^{ij} \approx 0$, which determine the 6 Lagrange multipliers $\hat\Phi_{ij}$ (if one is in the gravitational sector. In the topological sector, one gets tertiary constraint with yet more degrees of freedom.)

\end{description}

\noindent To recapitulate, we start with a phase space which has 72 degrees of freedom per point on $\Sigma$.   There are a total of 54 constraints in the gravitational sector, 14 of which are first class.  This gives us gives us the correct counting of a 4 dimensional reduced phase space per point.

\vspace{1cm}

\noindent Now, in this and previous analyses, we have reduced by the following constraints while still in the continuum setting:
\be
\label{pleb11}
\Phi(N_i,N_j),\; \Phi(N_i,\Pi^j),\; \Phi(N_i,P^j),\; \Phi(\Pi^i,P^j),\; \kappa_0,\; \kappa_i.
\ee
These are 32 constraints, 4 of which are first class.  The effect of imposing such constraints has been laid bare in \cite{henneaux}.  The 14 equations $\Phi(N,N)$ and $\Phi(N,\Pi)$ determine 14 of the 18 components of $N_i{}^A$.  They leave 4 free, essentially the lapse $\cN$ and the shift $\cN^i$.  In other words, they allow us to determine $N_i^A$ in terms of $\Pi^i_A$, $\cN$ and $\cN^i$.  The 14 constraints $\Phi(N, P)$ and $\Phi(\Pi,P)$ kill 14 of the 18 components of $P^i{}_A$.  The final 4 components are killed by $\kappa_0$ and $\kappa_i$.  But these are first class constraints, so we should introduce gauge-fixing conditions. What is particularly nice, is that  $\kappa_0$ and $\kappa_i$ are the canonical momenta to the lapse and shift.  Thus, they generate arbitrary shifts in these functions and we may supplement this constraint set with 4 conditions fixing $\cN$ and $\cN^i$.   

Reducing by these constraints effectively removes $P^i{}_A$ and $\cP_\g N_i{}^A$ as independent variables from the theory.  This leaves us with $w_i{}^A$ and $\cP_\g\Pi^i{}_A$ as the remaining phase space variables, 36 in total and once again the correct counting. However, in reducing by second class constraints (or gauge-fixed first class constraints), one must take care of the symplectic structure on the constraint hypersurface. We present the details of this calculation for the interested reader in Appendix \ref{red}.  Luckily, it turns out that symplectic structure among the remaining independent variables is left unchanged by the reduction process, that is:
\be
\label{pleb12}
\ba{rcl}
\{w_i{}^A, \cP_\g\Pi^j{}_B\}_D &=& \{w_i{}^A, \cP_\g\Pi^j{}_B\},\\[0.2cm]
\{\cP_\g\Pi^i{}_A, \cP_\g\Pi^j{}_B\}_D &=& \{\cP_\g\Pi^i{}_A, \cP_\g\Pi^j{}_B\},\\[0.2cm]
\{w_i{}^A, w_j{}^B\}_D &=& \{w_i{}^A, w_j{}^B\}
\ea
\ee
It is high time that we discretized the theory, but first, we shall replace the secondary simplicity constraint by an equivalent expression:
\be
\label{pleb13}
\Psi{}^{ij}  \approx  \epsilon^{mn(i} <h_{mp}\; \cP_\g\Pi^p, D_n\Pi^{j)} >, 
\ee
where $h_{ij}$ is the spatial metric.  It is defined by: $h h^{ij} =\; < \Pi^i,\Pi^j>$, $h = \det (h_{ij})$ and $h^{ij}$ is the inverse of $h_{ij}$.    As one can see from \eqref{red08}, it is a trivial consequence of the gauge $\cN = \sqrt{h}$, $\cN^i = 0$, but one can show that it is a gauge-invariant statement \cite{henneaux}.

\vspace{3cm}

First let us reduce by: 
\be
\label{red01}
\Phi(N_i,N_j),\; \Phi(N_i,\Pi^j),\; \Phi(N_i,P^j),\; \Phi(\Pi^i,P^j).
\ee
These form a second class set of 28 equations.  The Dirac matrix and its inverse have the block form:
\be
\label{red02}
I = 
\left(\ba{cccc}
0 & 0 & 0 & A\\[0.2cm]
0 & 0 & B & 0\\[0.2cm]
0 & -B^T & 0 & C\\[0.2cm]
-A^T & 0 & -C^T & 0
\ea\right), \quad\quad\quad 
I^{-1} = 
\left(\ba{cccc}
0 & -(A^{-1})^TC^TB^{-1} & 0 & -(A^{-1})^T\\[0.2cm]
(B^{-1})^TCA^{-1} & 0 & -(B^{-1})^T & 0\\[0.2cm]
0 & B^{-1} & 0 & 0\\[0.2cm]
A^{-1} & 0 & 0 & 0
\ea\right).
\ee
Since $\cP_\g\Pi^i{}_A$ commutes with all the above constraints, one has immediately that:
\be
\label{red03}
\{w_i{}^A, \cP_\g\Pi^j{}_B\}_I = \{w_i{}^A, \cP_\g\Pi^j{}_B\} \quad\quad \textrm{and}\quad\quad
\{\cP_\g\Pi^i{}_A, \cP_\g\Pi^j{}_B\}_I = \{\cP_\g\Pi^i{}_A, \cP_\g\Pi^j{}_B\}.
\ee
On the other hand $w_i{}^A$ has non-trivial commutation relations with $\Phi(N_i,\Pi^j)$ and $\Phi(\Pi^i,P^j)$. This means however, that the only blocks arising in the definition of the new bracket are $I^{-1}{}_{22},\, I^{-1}{}_{24},\, I^{-1}{}_{42}$ and $I^{-1}{}_{44}$ which are all zero, so:
\be
\label{red04}
\{w_i{}^A, w_j{}^B\}_I = \{w_i{}^A, w_j{}^B\}.
\ee

\vspace{1cm}

\noindent We next turn our attention to the first class constraints: $\kappa_0$ and $\kappa_i$.  As we mentioned in the main text, they generate transformations of the lapse and shift functions, so that we may gauge-fix by stipulating conditions on $\cN$ and $\cN^i$.  For this purposes, it would be nice to have a definition of $\cN$ and $\cN^i$ in terms of $N_i{}^A$ and $\cP^i{}_A$.  

To accomplish this, let us begin with the definition of the spatial metric $h_{ij}$:
\be
\label{red05}
h\,h^{ij} =\; <\Pi^i, \Pi^j>,
\ee
where $h=\det(h_{ij})$ and $h^{ij}$ is the inverse spatial metric. Then, notice that  $\Pi^i{}$ and $\epsilon(\Pi^i)$ provide a basis for the 6-dimensional space of bi-vectors. With this in mind, one can introduce projectors:
\be
\label{red06}
\cP_{\delta}{}^{AB} := h^{-1}\; h_{ij}\;   \Pi^{i}{}^{A}\; \Pi^j{}^B
\quad\quad\textrm{and}\quad\quad
\cP_{\epsilon}{}^{AB} := h^{-1}\; h_{ij}\;  \epsilon(\Pi^i){}^A\; \epsilon(\Pi^j){}^B.
\ee
They project onto $\Pi^i$ and $\epsilon(\Pi^i)$, respectively, and satisfy:\footnote{Although we do not need it here,  they are orthogonal once $\Phi(\Pi,\Pi)$ is imposed.}
\be
\label{red07}
\cP_{\delta}{}^{AB} + \cP_{\epsilon}{}^{AB} = \delta^{AB}.
\ee
Using this property:
\be
\label{red08}
N_i{}^A = \frac12\cN h^{-\frac12}h_{ij}  \epsilon(\Pi^j)^A  + \frac12\epsilon_{ijk}\cN^j \Pi^{kA} 
\quad\quad\textrm{where}\quad\quad
\ba{rcl} 
\cN &:=& \frac{2}{3}h^{-\frac12} \prec \Pi^i, N_i\succ,\\[0.2cm]
\cN^i &:=& \epsilon^{ijk} <h^{-1}h_{jl}\Pi^l,N_k>
\ea
\ee
and we used $\Phi(N,N)$ and $\Phi(N,\Pi)$ to simplify expressions, for example, to show that $<N_{(i},h_{j)k} \Pi^k> = 0$.
The definitions of lapse and shift may look rather complicated but one can show that in the gravitational sector:
\be
\label{red09}
\left(
\ba{cc}
\cN^2+ h_{ij}\cN^i\cN^j &  \cN^ih_{ij}\\[0.2cm]
h_{ij}\cN^j & h_{ij} 
\ea
\right)
 = \delta_{ab}\; e_\mu{}^{a}\; e_{\nu}{}^b ,
\ee
which is in agreement with the standard decomposition of the metric.  Now, let us consider the second class system:
\be
\label{red10}
\kappa_0,\; \kappa_i,\; \nu^i,\; \nu^0,
\ee
where $\nu^0 = \cN-1$ and $\nu^i = \cN^i$.  The Dirac matrix and its inverse are:
\be
\label{red11}
D = 
\left(\ba{cccc}
0 & 0 & 0 & 1\\[0.1cm]
0 & 0 & \I_{3\times 3} & 0\\[0.1cm]
0 & -\I_{3\times 3} & 0 & 0\\[0.1cm]
-1 & 0 & 0 & 0
\ea\right), \quad\quad\quad 
D^{-1} = 
\left(\ba{cccc}
0 & 0 & 0 & -1\\[0.1cm]
0 & 0 & -\I_{3\times 3} & 0\\[0.1cm]
0 & \I_{3\times 3} & 0 & 0\\[0.1cm]
1 & 0 & 0 & 0
\ea\right).
\ee
Once again, it is a trivial matter that the $\cP_\g\Pi^i$ part of the symplectic structure is left unchanged. It is not so trivial anymore to show that $\{w_i{}^A,w_j{}^B\}_D = 0$ but with a very small amount of investigation, one can easily see that  $\{w_i{}^A,\nu^j\} \approx 0 \approx \{w_i{}^A,\nu^0\}$.  Thus, given the form of $D^{-1}$, this implies the hoped for result.  Thus, one ends up with:
\be
\label{red12}
\ba{c}
\{w_i{}^A, \cP_\g\Pi^j{}_B\}_D = \{w_i{}^A, \cP_\g\Pi^j{}_B\}, \quad\quad 
\{\cP_\g\Pi^i{}_A, \cP_\g\Pi^j{}_B\}_D = \{\cP_\g\Pi^i{}_A, \cP_\g\Pi^j{}_B\} \\[0.2cm]
 \{w_i{}^A, w_j{}^B\}_D = \{w_i{}^A, w_j{}^B\}.
 \ea
\ee
